# Supplementary material for: Antiferromagnetic bosonic $t$-$J$ models and their quantum simulation in tweezer arrays
Source: arXiv:2305.02322 source file (2024-06-04)

a) Bosons

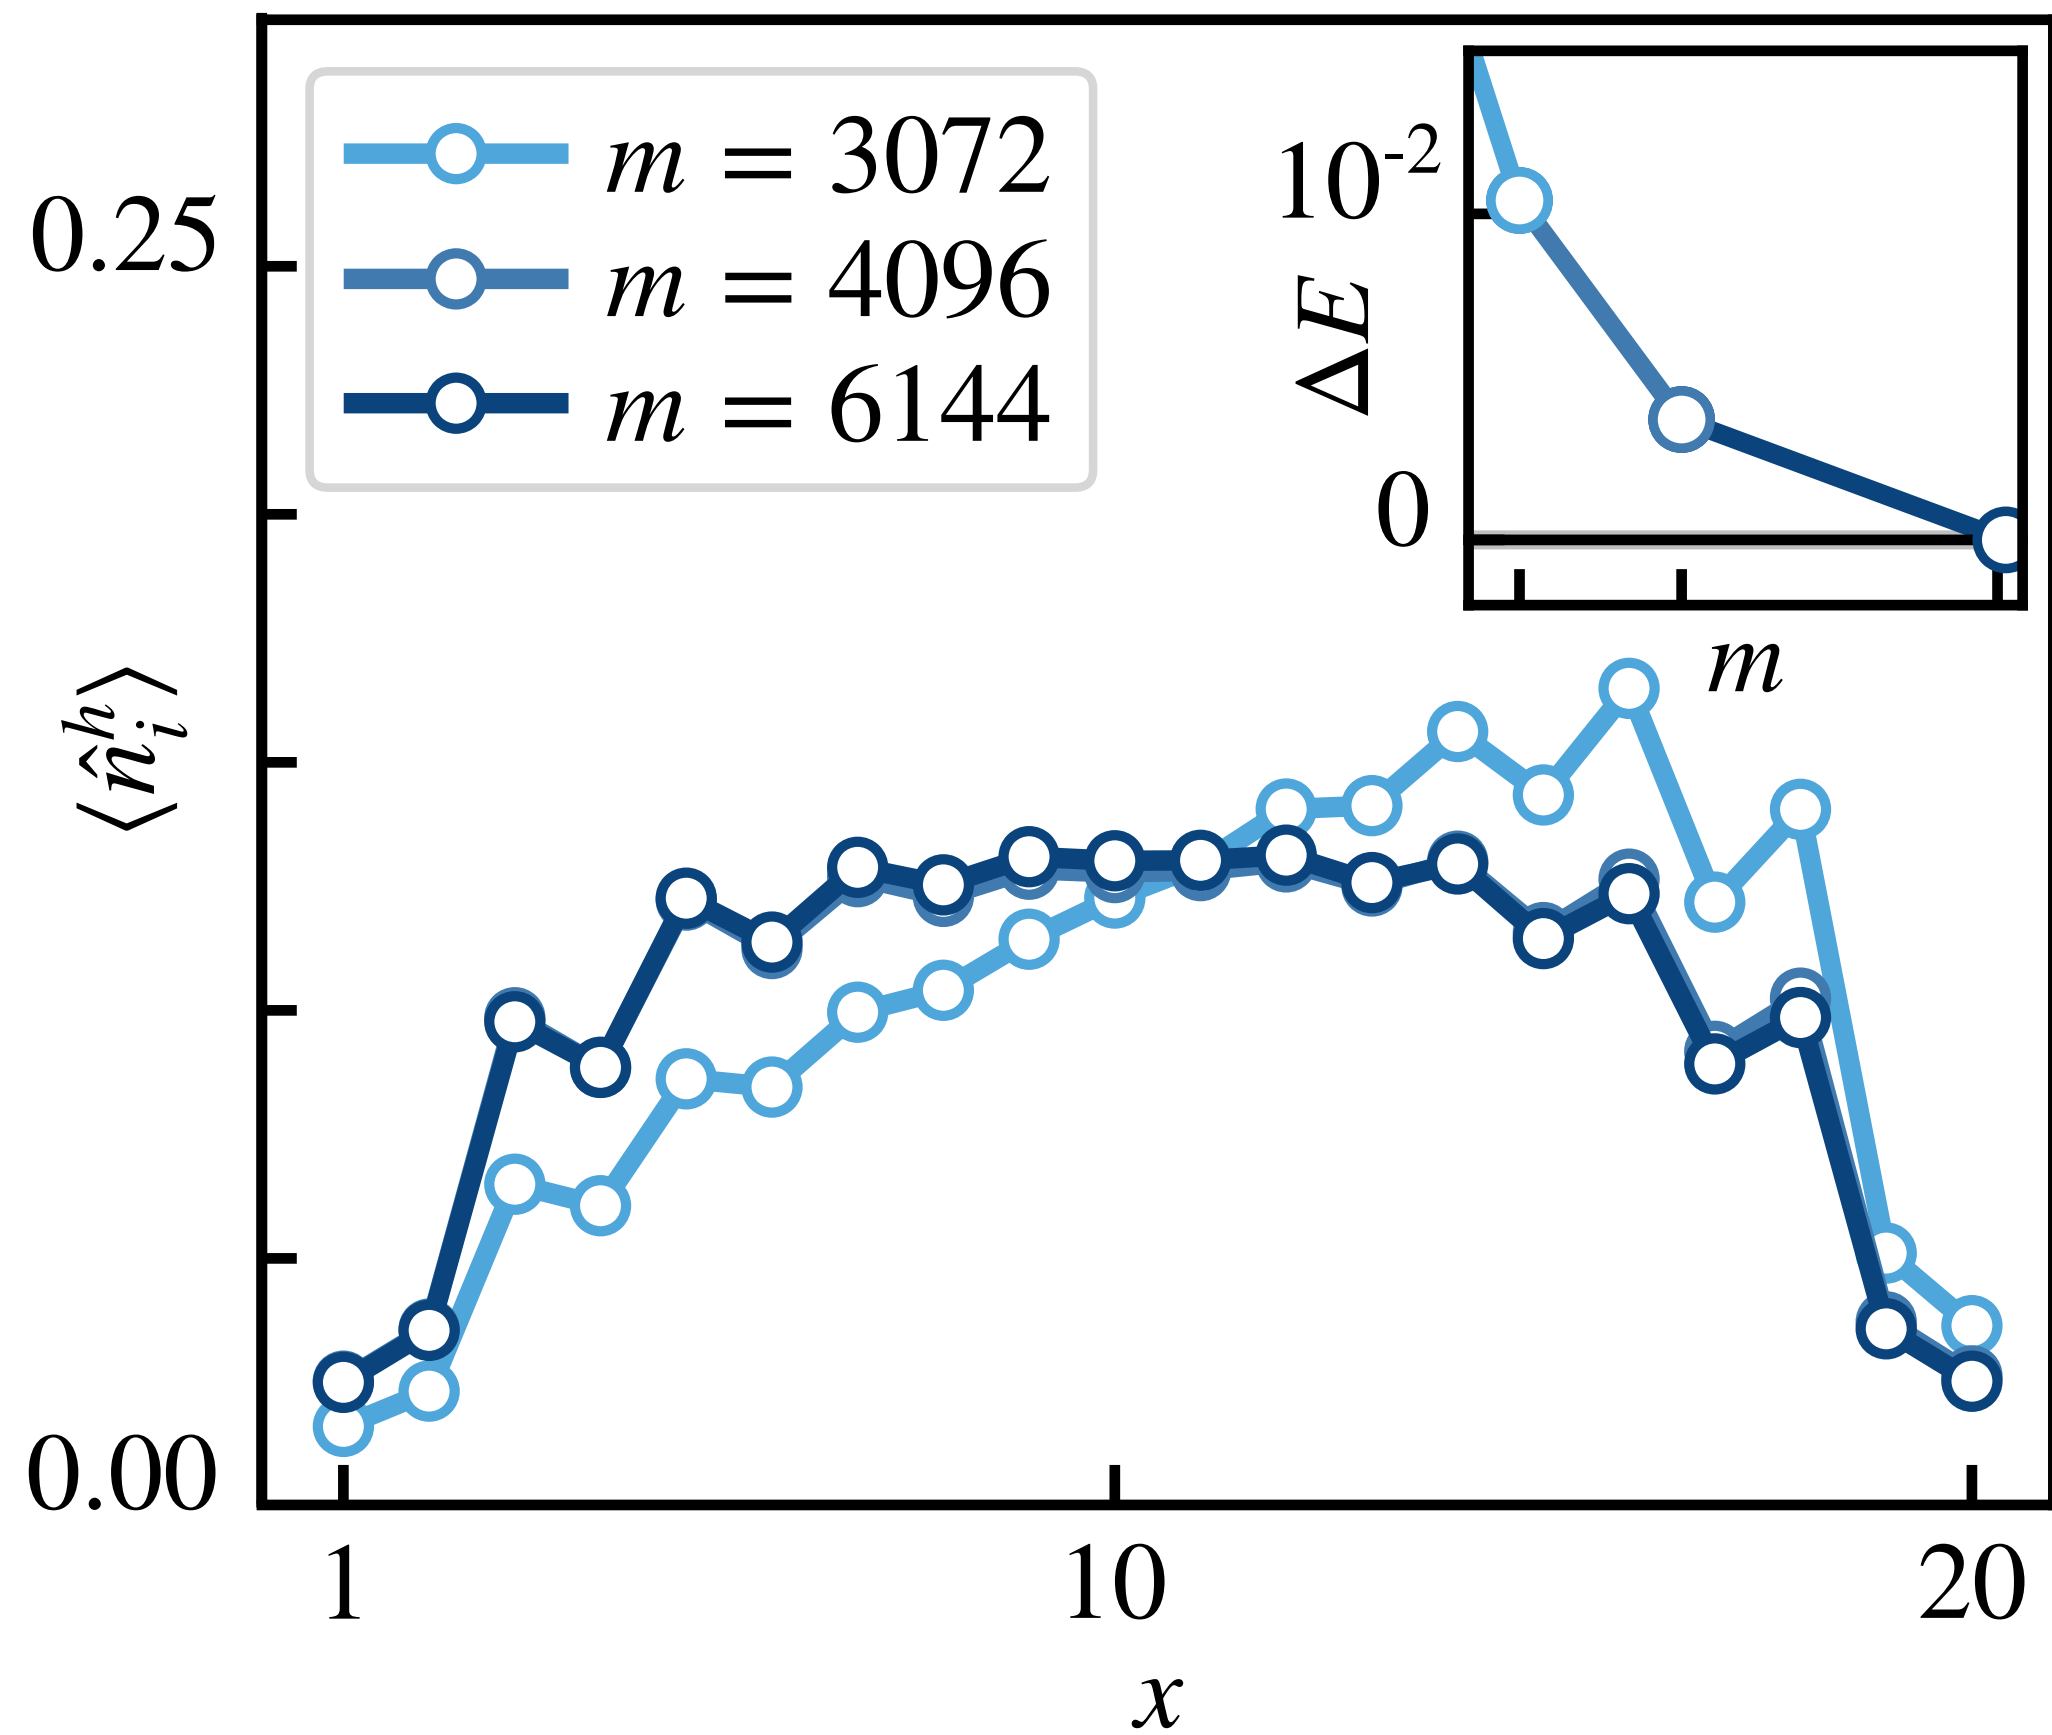

b) Fermions

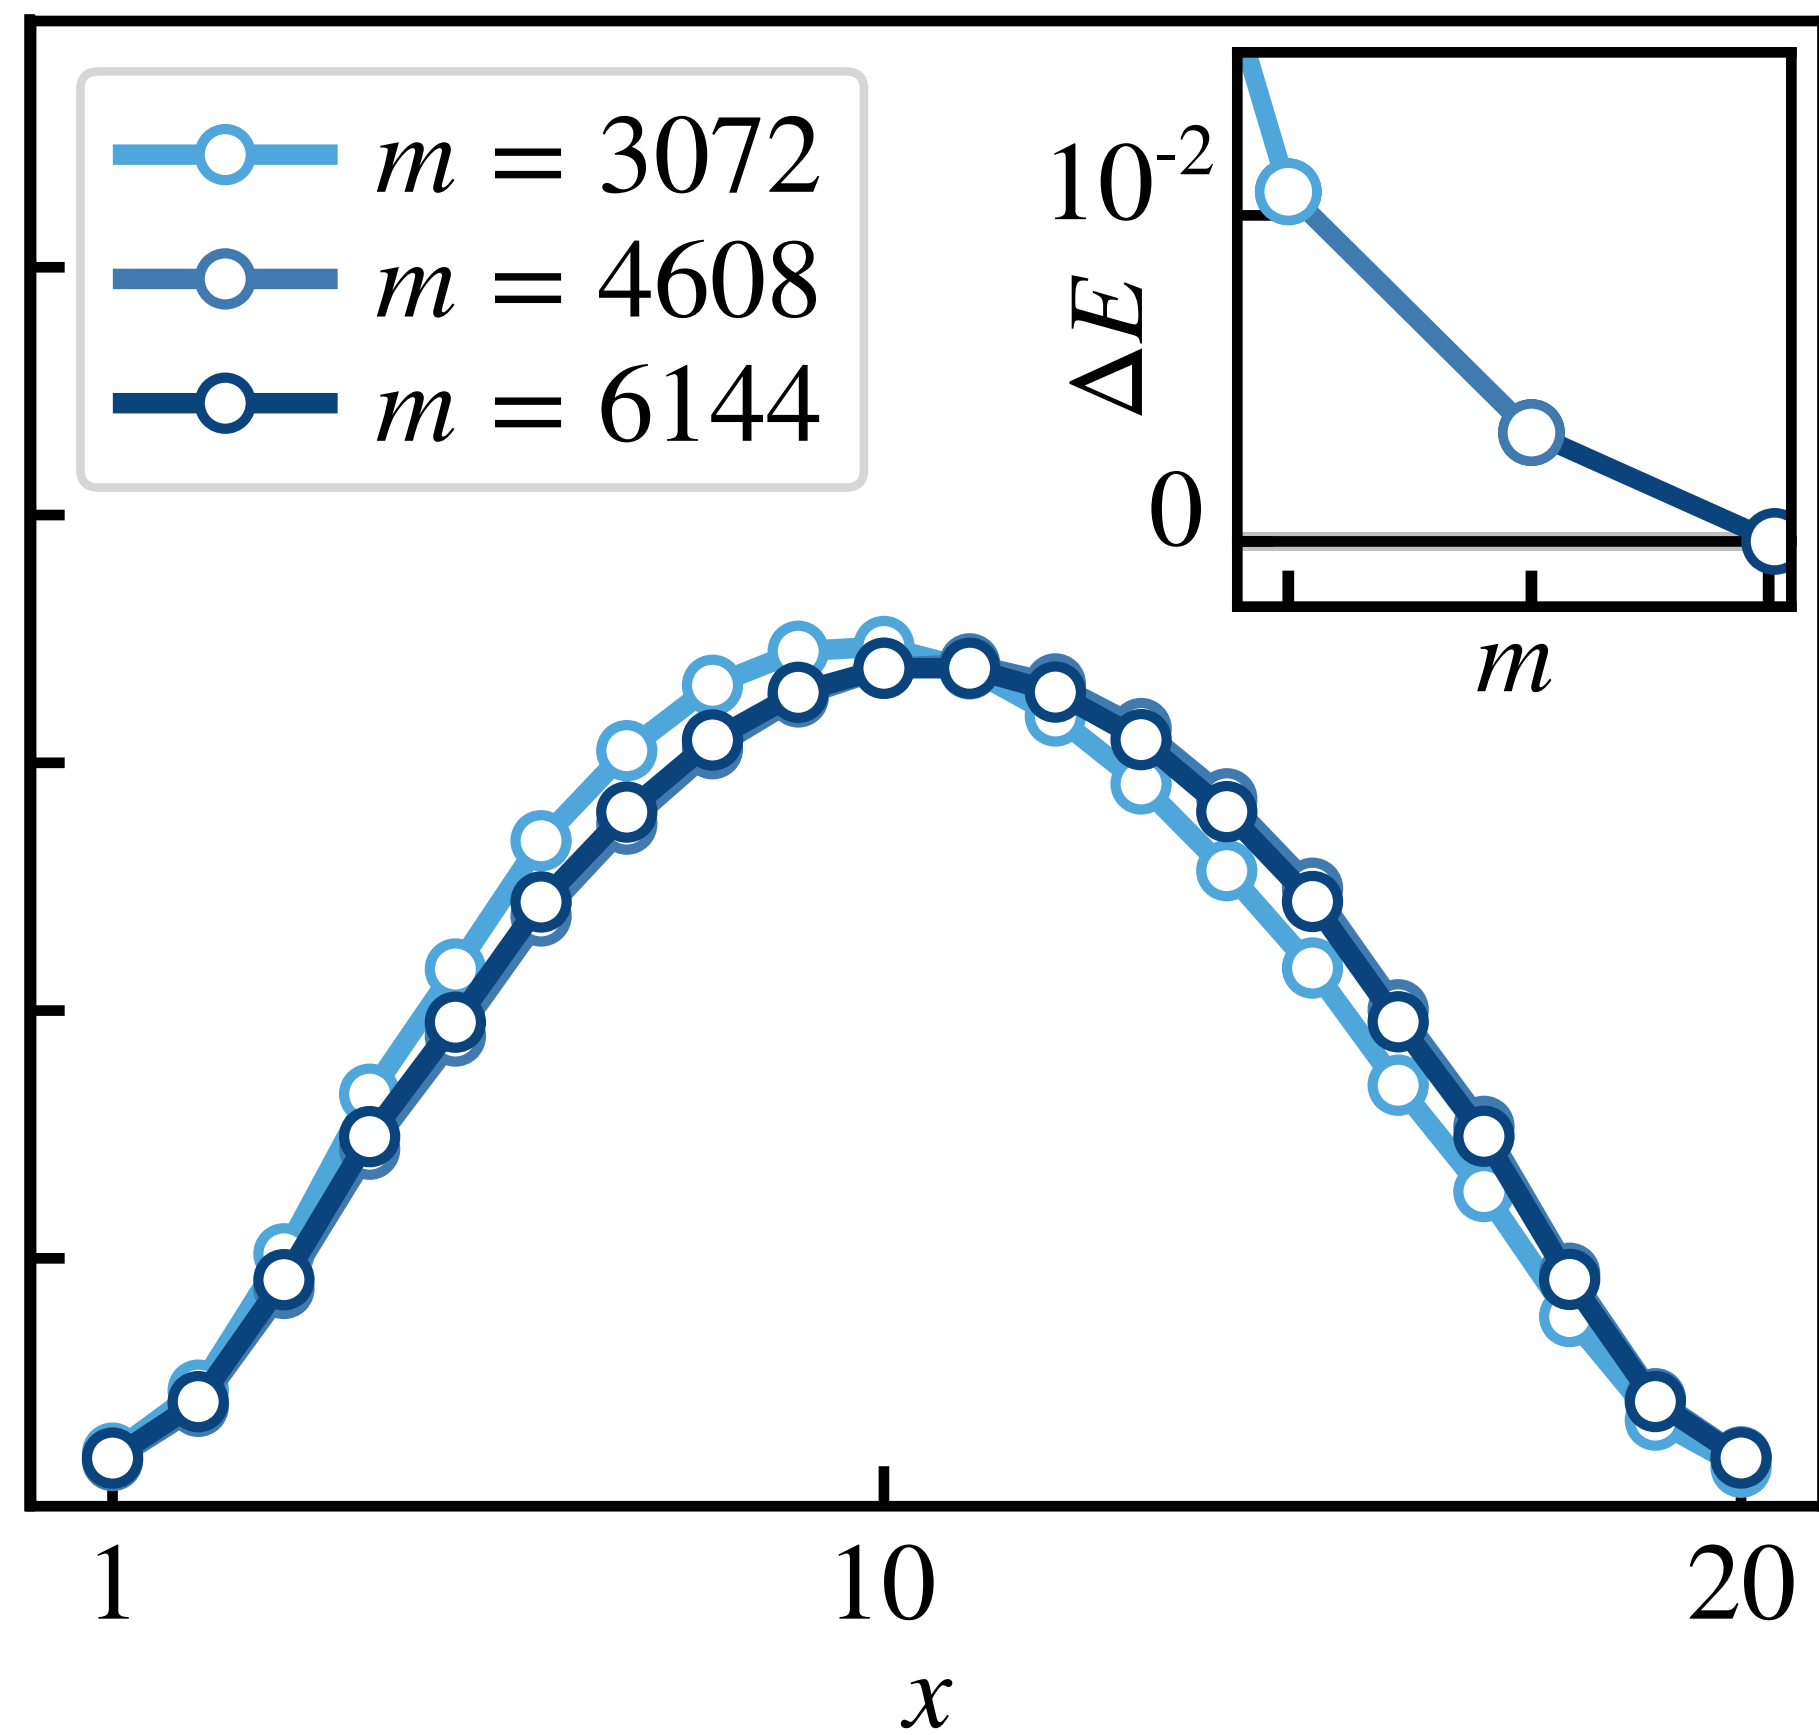

Supplement: Supplementary file 1 [file figSupp_convergence.pdf]
